# Supplementary material for: Fast Failure Recovery for Main-Memory DBMSs on Multicores
Source: arXiv:1604.03226 source file (2017-03-22)
Supplement: Supplementary file 1 [file appendix-chopping.tex]

\section{Transaction Chopping}
\label{sec:chopping}

In the database literature, transaction chopping~\cite{shasha1995transaction} has been
used to partition large transactions into a collection of pieces
for reduced lock contentions in transaction execution. 
By constructing SC-graph for transactions
prior to execution, transaction chopping resorts to
certain concurrency control mechanism, such as timestamp
ordering or two-phase locking, for serializing transactions.
This pure static analysis, unfortunately, violates the ordering constraints
in failure recovery. In fact, even if the ordering constraints
can be satisfied through order-preserving protocol,
this approach still leads to very coarse-grained decomposition
with much fewer opportunities to exploit parallelism.

\begin{figure}[ht!]
        \centering
        \subfloat[Transaction chopping.]{
                \includegraphics[width=0.45\columnwidth]{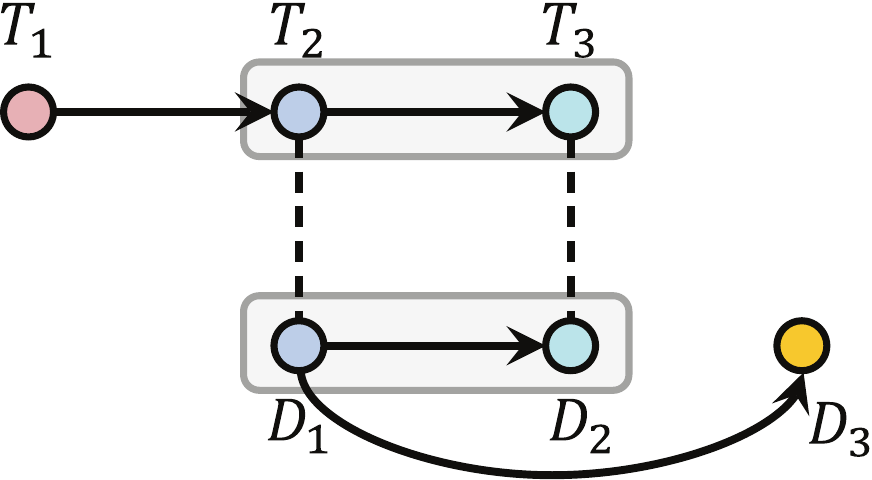}
                \label{fig:cmp-chop}
        }
        \subfloat[Static analysis in \system.]{
                \includegraphics[width=0.45\columnwidth]{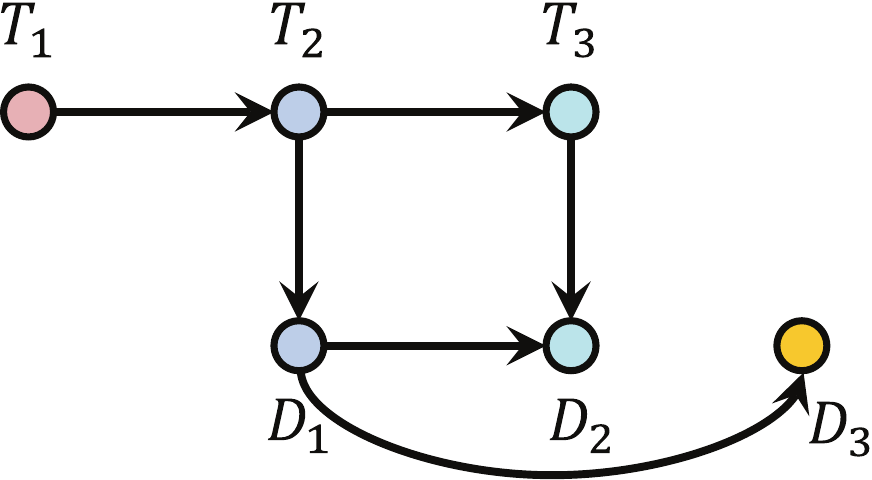}
                \label{fig:cmp-slice}
        }
        \caption{A comparison between transaction chopping and static analysis in \system. 
        In (a), solid lines stand for S-edges, and dashed lines stand for C-edges. 
        Transaction chopping serializes transactions at runtime and generates coarse-grained partitions. 
        \system determines the replay order prior to transaction re-execution 
        and generates finer-grained decomposition.}
\end{figure}

Let us reconsider the banking examples in \cref{fig:banktransferslice} and \cref{fig:bankbonus}. 
Transaction chopping conservatively merges $T_2$ and $T_3$, $D_1$ and $D_2$ into two \textit{super pieces}, 
due to the existence of a large SC-cycle, as shown in \cref{fig:cmp-chop}.
With the constructed SC-graph, transaction chopping resorts to certain concurrency control protocol, 
such as two-phase locking, to explore concurrency and serialize transactions at runtime. 
However, such a mechanism cannot guarantee ordering, which is required for failure recovery.
\system in contrast designs its static analysis specifically for order-preserving re-execution, 
where transactions are replayed following a strict order.
With this ordering guarantee, the static analysis in \system no longer needs to 
keep track of the conflicts among transactions, 
so that finer-grained program decomposition can be generated. 
As shown in \cref{fig:cmp-slice}, the execution order of $T_2$, $T_3$, $D_1$, and $D_2$ 
are decided before processing, 
thus piece merging is no longer required in \system's static analysis.
With the help of dynamic analysis, 
\system extracts high degree of parallelism by relaxing the ordering constraints at runtime.
